# Supplementary material for: Cortex: A Compiler for Recursive Deep Learning Models
Source: arXiv:2011.01383 source file (2021-03-05)
Supplement: Supplementary file 1 [file appendix.pdf]

# APPENDIX FOR CORTEX: A COMPILER FOR RECURSIVE DEEP LEARNING MODELS

## A ILIR LOWERING

### A.1 Uninterpreted Functions

The ILIR extends a tensor compiler to support indirect memory accesses and variable loop bounds. During code generation, CORTEX therefore has to handle expressions involving such uninterpreted functions. In order to perform simplification over such expressions, for purposes such as proving if certain bound checks are redundant, we use the Z3 SMT solver (De Moura & Bjørner, 2008).

### A.2 Bounds Inference

We briefly mentioned how in a traditional tensor compiler, there is a one-to-one relationship between the dimensions of a tensor and the loops in the corresponding operator’s loop nest<sup>1</sup>. This can be seen in Fig. A.1. In the figure, two loops, each corresponding to a dimension of the tensor  $r$  are generated in IR (shown in the generated code on the right).

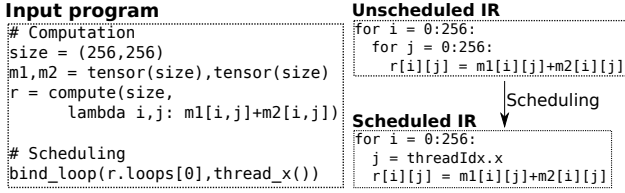

Figure A.1: Element-wise matrix addition in a tensor compiler

We also saw how in the ILIR, this relationship needs to be explicitly specified. We do this by the way of *named dimensions*. Named dimensions are identifiers associated with tensor dimensions and loops, which allow us to explicitly specify and keep track of relationships between loops and tensor dimensions. Consider the ILIR in Listing A.1 which shows the named dimensions annotated as comments. The dimensions of the tensor  $rnn$  are labeled with the named dimensions  $d\_node$  and  $d\_hidden$ . The tensor index dimension  $d\_node$  corresponds to the two loop dimensions  $d\_all\_batches$  and  $d\_batch$ .

Named dimensions also make the semantic meaning of loops and index expressions explicit. For example, the

<sup>1</sup>We do not cover the case of optimizations such as loop splitting which give rise to additional loops here for brevity. Similarly, operators involving reduction are not covered here.

```

1 # rnn[node_dim, hidden_dim]
2 L1: for n_idx = 0:leaf_batch_size: # d_batch
3     node = leaf_batch[n_idx]
4 L2: for i = 0:256:
5     rnn[node,i] = Emb[words[node],i]
6
7 L3: for b_idx = 0:num_internal_batches: # d_all_batches
8 L4: for n_idx = 0:batch_sizes[b_idx]: # d_batch
9     node = internal_batches[b_idx,n_idx]
10 L5: for i = 0:256: # d_hidden
11     lh[node,i] = rnn[left[node],i]
12 L6: for i = 0:256: # d_hidden
13     rh[node,i] = rnn[right[node],i]
14 L7: for i = 0:256: # d_hidden
15     rnn[node,i] = tanh(lh[node,i] + rh[node,i])

```

Listing A.1: ILIR generated for the model in Fig. 1

first dimension of the tensor  $rnn$  is labeled  $d\_node$  and corresponds to the space of all nodes. It, therefore, does not make sense to index  $rnn$  by  $b\_idx$ , the loop variable for the loop associated with  $d\_all\_batches$ .

### A.3 Caching Tensors Indexed by Non-Affine Expressions

We saw in §5.1 how when an intermediate tensor is stored in scratchpad memory, it can be better to index it by the dense contiguous loop iteration space as opposed to the sparse index space of the original tensor. A similar situation occurs when a caching a tensor accessed by multiple non-affine index expressions. Assume, for example, if we wished to cache the tensor  $rnn$  in loop L4 in Listing A.1, for the purposes for the accesses  $rnn[left[node], i]$  and  $rnn[right[node], i]$ . We create a cached tensor with an additional dimension corresponding to the multiple non-affine index expressions, as shown in the listing below.

```

1 for b_idx = 0:num_internal_batches:
2   for n_idx = 0:batch_sizes[b_idx]:
3     node = internal_batches[b_idx,n_idx]
4     for i = 0:256:
5       rnn_cache[b_idx,n_idx,i,0] = rnn[left[node],i]
6       rnn_cache[b_idx,n_idx,i,1] = rnn[right[node],i]
7
8   for b_idx = 0:num_internal_batches:
9     for n_idx = 0:batch_sizes[b_idx]:
10      node = internal_batches[b_idx,n_idx]
11      for i = 0:256:
12        rnn[node,i] = tanh(rnn_cache[b_idx,n_idx,i,0] +
13                           rnn_cache[b_idx,n_idx,i,1])

```

### A.4 Barrier Insertion

We need to insert synchronization barriers and memory fences when threads read data written by other threads. This is true on CPUs as well as on accelerators such as

GPUs. The barrier insertion pass in TVM does well on tensor programs that do not have loop-carried dependencies. Specifically, given a loop-carried dependence, the pass conservatively places barriers in the innermost loop, as opposed to placing it in the body of the loop that actually carries the dependence. This can lead to unnecessary barriers, leading to inflated runtimes.

As we iterate sequentially either over data structure nodes (when dynamic batching is not performed) or batches of nodes (when dynamic batching is performed), the data dependencies between a node and its children manifest as loop-carried dependencies in the generated ILIR code. This can be seen in the generated ILIR for the running example, in Listing A.1. In the listing, the data written to tensor `rnn` in loops `L2` and `L7` is read by loops `L5` and `L6`. This dependence only exists across a node and its children. We are also guaranteed, by the properties described in §2 and the way the data structure linearizer works, that no node in batch may be a child of any other node in the same batch. The, therefore, dependence is carried by loop `L3`, and not by loop `L4`.

Given this dependence, we would need a barrier at the start of every iteration of loop `L3`. However, the conservative barrier insertion pass in TVM instead places a barrier in the body of loop `L3`. We therefore designed a modification to the pass to insert the barrier in the outer loop which actually carries the dependence.

#### A.5 Other Optimizations during ILIR Lowering

Below, we discuss a couple less important optimizations and scheduling knobs we implemented.

**Loop Peeling:** The generated ILIR in CORTEX involves loops with variable loop bounds. Splitting such loops gives rise to bounds checks in the bodies of the loops. We employ loop peeling to ensure that such checks are only employed for the last few iterations of the loop.

**Rational Approximations of Nonlinear Functions:** We use rational approximations for the *tanh* and *sigmoid* functions which makes exploiting SIMD instructions on CPUs easier.

## B DATA STRUCTURE LINEARIZATION

In our data structure linearizers, when lowering a pointer linked data structure to arrays, we associate the nodes with integer identifiers. When doing so for the case of dynamic batching, we ensure that nodes in a batch are numbered consecutively and higher than their parents. This allows us to lower the batches into two arrays — `batch_begin` and `batch_length`, which store the starting node and the length, respectively, of every batch.

Thus, node `n` is in batch `i` if `batch_begin[i] ≤ n < batch_begin[i] + batch_length[i]`. This numbering scheme also ensures that all leaf nodes are numbered higher than all internal nodes. This reduces the cost of checking if a node is a leaf. When nodes are numbered this way, a leaf check involves a single comparison as opposed a memory load (to load the number of children of a node under question, for example) and a comparison in the case where the numbering is arbitrary. This scheme thus generally reduces the overheads of iterating over batches and leaf checks.

## C REGISTER PRESSURE IN CUDA

CORTEX generated CUDA kernels are often large, due to optimizations such as aggressive kernel fusion, loop peeling, loop unrolling and recursive unrolling. Furthermore, model persistence uses GPU registers to persist model weights. These factors leads to high register pressure. We find that recursive unrolling precludes us from using persistence for the TreeLSTM and TreeRNN models discussed in §7.4. Similarly, we note that we cannot apply the loop peeling and model persistence optimizations in the case of the TreeLSTM model at the same time. In our schedules, we have explored this trade-off space and evaluated on the best performing schedule. We note that techniques developed in past work such as (Rawat et al., 2018) and (Sakdhnagool et al., 2019) can potentially be applied in our context to alleviate this issue.

## REFERENCES

- De Moura, L. and Bjørner, N. Z3: An efficient smt solver. In *International conference on Tools and Algorithms for the Construction and Analysis of Systems*, pp. 337–340. Springer, 2008.
- Rawat, P. S., Rastello, F., Sukumaran-Rajam, A., Pouchet, L.-N., Rountev, A., and Sadayappan, P. Register optimizations for stencils on gpus. In *Proceedings of the 23rd ACM SIGPLAN Symposium on Principles and Practice of Parallel Programming*, PPOPP ’18, pp. 168–182, New York, NY, USA, 2018. Association for Computing Machinery. ISBN 9781450349826. doi: 10.1145/3178487.3178500. URL <https://doi.org/10.1145/3178487.3178500>.
- Sakdhnagool, P., Sabne, A., and Eigenmann, R. Regdem: Increasing GPU performance via shared memory register spilling. *CoRR*, abs/1907.02894, 2019. URL <http://arxiv.org/abs/1907.02894>.
